# Supplementary material for: Carrier-envelope phase control over pathway interference in strong-field dissociation of H$_2^+$
Source: arXiv:1306.4010 ancillary file (2013-06-17)
Supplement: Supplementary file 1 [file SuppMat.pdf]

# Theoretical background

## I. SOLVING THE TIME-DEPENDENT SCHRÖDINGER EQUATION

We solved the time-dependent Schrödinger equation for the total $H_2^+$ wave function including nuclear and electronic degrees of freedom as described in Ref. [1]. We will very briefly summarize the salient points here.

The laser field was taken to be

$$\mathcal{E}(t) = \mathcal{E}_0 e^{-t^2/\tau^2} \cos(\omega t + \varphi). \quad (1)$$

where $\tau$ is related to the full width of the intensity at half maximum $\tau_{\rm FWHM}$ by $\tau = \tau_{\rm FWHM}/\sqrt{2\ln 2}$, $\omega$ is the carrier frequency, and $\varphi$ is the CEP. The wave function was expanded on products of Born-Oppenheimer electronic states and Wigner $D$-functions representing the nuclear rotation. The calculations thus include nuclear vibration and rotation as well as electronic excitation. The primary physical process excluded is ionization, which limits the maximum intensities we can treat.

Testing that included the $n = 2$ manifold showed that dissociation to this excited manifold of states amounted to 0.45% of the total dissociation probability at the highest intensity where it takes its largest value. In fact, we used this probability to determine the maximum intensity we considered — based on our relative accuracy goal of 1% — under the assumption that it serves as a good proxy for the ionization probability. We further compared the asymmetry calculated with both the $n = 1$ and the $n = 2$ manifolds to the asymmetry calculated with only the $n = 1$ manifold. At the highest intensity, there was a 10% relative difference between the two. This error, however, was by far the largest in our calculation since we ensured that the asymmetry was converged to at least two digits with respect to all other parameters of the calculation. The $n = 2$ manifold was included for intensities above $10^{13}$ W/cm$^2$.

## II. CALCULATING THE PHYSICAL OBSERVABLES

The fundamental physical observable is the $p$+H relative momentum distribution which we will obtain as a KER-$\cos\theta_K$ distribution. Calculating this distribution correctly [2, 3] involves projecting the final wave function onto scattering states that behave as $\exp(i\mathbf{K}\cdot\mathbf{R})\phi_{1sA}$ asymptotically, where $\mathbf{R}$ points from proton $A$ to proton $B$ and $\phi_{1sA}$ is the hydrogen ground state wave function centered on proton $A$. The momentum $\mathbf{K}$ thus points from H to $p$. This scattering state, with the nuclear spin included, is then symmetrized to account for the identical nuclei [2, 4, 5]. Carrying out these steps, the KER-$\cos\theta_K$ distribution — with $E = K^2/2\mu$ the KER, $\mu$ the nuclear reduced mass, and $\theta_K$ the direction of $\mathbf{K}$ with respect to the polarization direction (labeled simply $\theta$ in the main text) — is

$$\frac{\partial^2 P}{\partial E \partial(\cos\theta_K)} = 2\pi \left| \sum_{J\,\text{even}} C_{Jg} Y_{J0}(\theta_K) + \sum_{J\,\text{odd}} C_{Ju} Y_{J0}(\theta_K) \right|^2 \quad (2)$$

with $(p = g, u)$

$$C_{Jp} = C_{Jp}(E) = (-i)^J e^{-i\delta_{Jp}} \langle EJp | F_{Jp}(t_f)\rangle \quad (3)$$

after specializing to a linearly polarized laser pulse assuming the initial state had $M = 0$. In this expression, $|F_{Jp}(t_f)\rangle$ are the $1s\sigma_g$ and $2p\sigma_u$ nuclear radial wave functions for total orbital angular momentum $J$ at the final time $t_f$, while $|EJp\rangle$ and $\delta_{Jp}$ are the corresponding energy-normalized scattering states and phase shifts, respectively. Note that the first term of Eq. (2) has even parity while the second has odd parity. It is when both terms contribute at the same energy, as determined by the CEP-dependent $C_{Jp}(E)$, that asymmetry will emerge [6].

For simplicity, we have not included a label in Eqs. (2) or (3) to indicate the initial state, but there will be separate distributions for each initial $v$. These $v$-dependent observables were then summed with weights given by the Franck-Condon factors as appropriate for an ion beam target [7]. These Franck-Condon-averaged observables were then further averaged over the laser's intensity distribution in the interaction region [7]. For the conditions of the experiment, the intensity averaging is accomplished for an observable $P(I)$ via the integral

$$\bar{P}(I_0) \propto \int_0^{I_0} P(I) \frac{dI}{I}. \quad (4)$$

Note that because intensity averaging emphasizes lower intensities over higher ones, the impact of the errors at the higher intensities due to the limited Born-Oppenheimer expansion is reduced. Comparing the intensity-averaged observables calculated with and without the $n = 2$ manifold, however, shows that the relative difference is generally reduced only marginally over the roughly 10% found without intensity averaging.

Equation (2) shows that although a linear combination of $1s\sigma_g$ and $2p\sigma_u$ is necessary to localize the electron as an atomic rather than a molecular state, the spatial asymmetry of $p$+H is due to the interference of even and odd nuclear parity states. Physically, the observable is the relative momentum of the nuclei, so it is their degrees of freedom that must be controlled. Of course, for simple homonuclear diatomic molecules like $H_2^+$, dipole selection rules and the need to project onto atomic states produce a close correspondence between the nuclear parity and the electronic state, making "electron localization" an alternative — but less general and less precise

— description for these systems. However, one need only consider heteronuclear diatomics, or possibly just more complicated homonuclear ones, to see that controlling the spatial asymmetry of the nuclear degrees of freedom is not generally equivalent to controlling electron localization. On the other hand, controlling the chemically distinguishable products of molecular dissociation without regard to their direction *is* equivalent to controlling electron localization.

## III. UNDERSTANDING THE ASYMMETRY

The pathway picture described briefly in the main text and proposed in Refs. [6, 8] is, in fact, an exact formulation of the problem that permits a simple physical interpretation of CEP effects. It also enables making simple, nontrivial predictions.

Following Ref. [6], the key observation is that the Hamiltonian is periodic in the CEP so the wave function must be as well. The wave function can then be conveniently — and exactly — expanded on a Fourier series in the CEP where the series' index can be interpreted as the *net* number of photons exchanged with the field. With this representation of the wave function, the CEP dependence of any physical observable can be analytically calculated. While Ref. [6] presented the expression so obtained for the asymmetry, it did so for non-rotating nuclei.

The full-dimensional expression — *i.e.*, including nuclear rotation — begins with the Fourier expansion of the time-dependent wave function in the KER-$\cos\theta_K$ distribution [Eq. (2)] over CEP,

$$\frac{\partial^2 P}{\partial E\partial(\cos\theta_K)} = 2\pi\left|\sum_{\substack{J\,\text{even}\\ n\,\text{even}}} C_{nJg}Y_{J0}(\theta_K)e^{in\varphi} + \sum_{\substack{J\,\text{odd}\\ n\,\text{odd}}} C_{nJu}Y_{J0}(\theta_K)e^{in\varphi}\right|^2 \quad (5)$$

with $(p = g, u)$

$$C_{nJp} = (-i)^J e^{-i\delta_{Jp}}\langle EJp|F_{nJp}(t_f)\rangle. \quad (6)$$

Equation (5) assumes that $J = 0$ initially since the dipole selection rules then guarantee that the number of photons $n$ is even (odd) if $J$ is even (odd).

The up and down probabilities used to define the asymmetry in Eq. (1) of the main text will typically involve an integration over some range of $\theta_K$, but we can understand the important structure by just considering the directions $\mathbf{K}$ and $-\mathbf{K}$ (or, equivalently, $\cos\theta_K$ and $-\cos\theta_K$, recalling that there is azimuthal symmetry about the laser polarization). Using the properties of the spherical harmonics, we can thus write the up ($u$) and down ($d$) probabilities as

$$\left.\frac{\partial^2 P}{\partial E\partial(\cos\theta_K)}\right|_{u,d} = 2\pi\left|\sum_{\substack{J\,\text{even}\\ n\,\text{even}}} C_{nJg}Y_{J0}(\theta_K)e^{in\varphi} \pm \sum_{\substack{J\,\text{odd}\\ n\,\text{odd}}} C_{nJu}Y_{J0}(\theta_K)e^{in\varphi}\right|^2. \quad (7)$$

After some algebraic simplification and suppressing the argument of $Y_{J0}$, the numerator of the normalized asymmetry $A(\text{KER},\varphi)$ is

$$\mathcal{A}(\text{KER},\varphi) = \left.\frac{\partial^2 P}{\partial E\partial(\cos\theta_K)}\right|_u - \left.\frac{\partial^2 P}{\partial E\partial(\cos\theta_K)}\right|_d = 4\pi\text{Re}\sum_{\substack{J\,\text{even}\\ n\,\text{even}}}\sum_{\substack{J'\,\text{odd}\\ n'\,\text{odd}}} C^*_{n'J'u}C_{nJg}Y_{J'0}Y_{J0}e^{i(n-n')\varphi}, \quad (8)$$

and the total dissociation probability in the denominator is

$$\begin{aligned}\mathcal{P}(\text{KER},\varphi) &= \left.\frac{\partial^2 P}{\partial E\partial(\cos\theta_K)}\right|_u + \left.\frac{\partial^2 P}{\partial E\partial(\cos\theta_K)}\right|_d \\ &= 2\pi\sum_{\substack{J\,\text{even}\\ n\,\text{even}}}|C_{nJg}Y_{J0}|^2 + 2\pi\sum_{\substack{J\,\text{odd}\\ n\,\text{odd}}}|C_{nJu}Y_{J0}|^2 \\ &+ 4\pi\text{Re}\sum_{\substack{J\,\text{even}\\ n\,\text{even}}}\sum_{\substack{J'\,\text{even}\\ n'\,\text{even}}} C^*_{n'J'g}C_{nJg}Y_{J'0}Y_{J0}e^{i(n-n')\varphi} \\ &+ 4\pi\text{Re}\sum_{\substack{J\,\text{odd}\\ n\,\text{odd}}}\sum_{\substack{J'\,\text{odd}\\ n'\,\text{odd}}} C^*_{n'J'u}C_{nJu}Y_{J'0}Y_{J0}e^{i(n-n')\varphi}. \end{aligned} \quad (9)$$

Equations (8) and (9) — which are exact — provide considerable insight into the origins of the CEP effects and their necessary conditions. Among other things, they show the following:

- The CEP dependence in $\mathcal{A}$ results from the interference of $n$-photon pathways that produce the same final $E$ at the same $\theta_K$ such that $\Delta n = n - n'$ is odd. That is, there is an asymmetry only when even and odd nuclear parities interfere since $J$ and $J'$ also satisfy $\Delta J = J - J'$ odd. Since it is much more likely that pathways differing by only one photon, $|\Delta n| = 1$, will contribute at the same final $E$ than it is for pathways with larger $|\Delta n|$, the dominant behavior of $\mathcal{A}$ will be $\cos(\varphi + \varphi_0)$.

- The CEP dependence in $\mathcal{P}$ also results from the interference of $n$-photon pathways that produce the same final $E$ at the same $\theta_K$ — except that $\Delta n$ is now even. Consequently, the dominant CEP dependence, $\cos(2\varphi + \varphi_0')$, results from the interference of pathways that differ by two photons. Since the likelihood that such pathways will contribute at the same final $E$ is much smaller than for $|\Delta n| = 1$, we expect CEP effects in $\mathcal{P}$ to be much smaller

than in $\mathcal{A}$, leaving primarily the CEP-independent $\Delta n = 0$ contribution. For sufficiently short pulses, however, $\mathcal{P}$ can have CEP dependence that contributes to the CEP dependence of the asymmetry.

- The only way that pathways with different net numbers of photons can produce the same final energy is for the laser bandwidth to be large. In fact, since the laser's power spectrum usually falls off exponentially, significant CEP effects in the asymmetry generally require the bandwidth to be around one-third or more of the energy at the central frequency, corresponding roughly to a three-cycle pulse or shorter. Because CEP effects arise from the overlap of exponential tails, their magnitude tends to grow exponentially with decreasing pulse length.

- All of the system's dynamics — indeed all reference to a specific system — is contained in the coefficients $C_{nJp}(E)$ as is all of the energy dependence. The energy-dependent tilt in $A(\mathrm{KER},\varphi)$ shown in Figs. 2 and 3 of the main text, for instance, arises from these coefficients, and $\varphi_0$ in $\mathcal{A}$ mentioned above can, in principle, be calculated from them.


[1] F. Anis and B. D. Esry, Phys. Rev. A **77**, 033416 (2008).

[2] F. Anis, Ph.D. thesis, Kansas State University, Manhattan, Kansas, U.S.A. (2009).

[3] F. Anis and B. D. Esry, Phys. Rev. Lett. **109**, 133001 (2012), URL http://link.aps.org/doi/10.1103/PhysRevLett.109.133001.

[4] T. A. Green and J. M. Peek, Phys. Rev. Lett. **21**, 1732 (1968).

[5] S. J. Singer, K. F. Freed, and Y. B. Band, J. Chem. Phys. **79**, 6060 (1983).

[6] J. J. Hua and B. D. Esry, J. Phys. B **42**, 085601 (2009).

[7] P. Q. Wang et al., Phys. Rev. A **74**, 043411 (2006).

[8] V. Roudnev and B. D. Esry, Phys. Rev. Lett. **99**, 220406 (2007).
